# Supplementary material for: Long Term Memory: The Foundation of AI Self-Evolution
Source: arXiv:2410.15665 source file (2025-05-11)
Supplement: Supplementary file 1 [file 07_appendix.tex]

\section{Autoencoder Details}
\label{sec:vae_details}

The training objective for our VAE closely follows that of \cite{esser2021taming}:
\begin{equation*}
\mathcal{L}_{\text{VAE}} = \mathcal{L}_1 + \mathcal{L}_{\text{LPIPS}} + 0.5 \mathcal{L}_{\text{GAN}} + 0.2 \mathcal{L}_{\text{ID}} + 0.000001 \mathcal{L}_{\text{KL}}
\end{equation*}
where $L_1$ is L1 loss in pixel space, $L_{\text{LPIPS}}$ is perceptual loss based on LPIPS similarity \cite{lpips}, $L_{GAN}$ is a patch-based discriminator loss, $L_{\text{ID}}$ is a perceptual loss based on internal features of the Moco v2 model \cite{chen2020improved}, and $L_{\text{KL}}$ is the standard KL-regularization term to encourage encoder outputs towards a normal distribution.
We delay the beginning of GAN training (i.e. including the adversarial loss in the loss function) to 50,000 steps, in order to let the VAE achieve sufficiently good reconstruction performance.
We use a latent dimension of 8.

The training objective for the VQ-GAN matches that of the VAE, with one notable exception: we replace the $\mathcal{L}_{\text{KL}}$ loss with the standard codebook commitment loss $\mathcal{L}_{\text{codebook}}$ \citep{vqvae}, which encourages encoder outputs and codebook vectors to be close together.
We use $\beta = 0.25$, and use loss weighting $1.0$.
The final loss function for the VQ-VAE is therefore:
\begin{equation*}    
\mathcal{L}_{\text{VQ-VAE}} = \mathcal{L}_1 + \mathcal{L}_{\text{LPIPS}} + 0.5 \mathcal{L}_{\text{GAN}} + 0.2 \mathcal{L}_{\text{ID}} + \mathcal{L}_{\text{codebook}}
\end{equation*}
The vector quantization layer is applied after projecting the encoder outputs to 8-dimensional space.
Outside of the loss function change and the quantization layer, the training setup for the VAE (for Transfusion) and VQ-VAE (for Chameleon) are the same (e.g. same amount of training compute, same training data, and same encoder/decoder architecture).



\section{Examples: Image Generation}
\label{sec:examples_image_generation}

Figure~\ref{fig:samples2} and Figure~\ref{fig:samples3} show examples of images generated from a 7B Transfusion model trained on 2T multi-modal tokens (\S\ref{sec:enhanced}).



\section{Examples: Image Editing}
\label{sec:examples_image_editing}

Figure~\ref{fig:edit2} show random examples of image editing by a fine-tuned 7B Transfusion model.
